# Supplementary material for: Learning compositionally through attentive guidance
Source: arXiv:1805.09657 source file (2019-07-05)
Supplement: Supplementary file 1 [file attention_mechanisms.tex]

\section{Attention mechanisms}
\subsection{MLP attention method}
The alignment model for the attention mechanism we use for all our final models is an multilayer perceptron that takes as input a decoder state ($do_t$) and an encoder state ($eo_i$), and calculates the score as:
$$
score(eo_i, do_t) = W_s * ReLU(W_c * [eo_i; do_t]),
$$

where $W_s$ is a $1 \times H$, and $W_c$ a $H \times 2H$ matrix. $H$ is the hidden layer size of the RNN.
We calculate these scores for every encoder state, and then use a softmax layer to transform the series of scores to a probability distribution.
The context vector is then computed as a weighted sum over the encoder states, taking the marginalised attention scores as weights:
$$
c_t(eo, do_t) = \sum_i eo_i * \frac{e^{score(eo_i, do_t)}}{\sum_j e^{score(eo_j, do_t)}}
$$

\subsection{Attention mechanisms}
We use two different attention mechanisms that differ in where the calculated context vectors are used in the decoder.

The first mechanism, which we call \textbf{post-rnn}, computes the attention scores based on the current decoder state $do_t$.
The context vector is then concatenated with $do_t$ and fed through the output layer of the network, that produces a probablity distribution over the output words:
$$
out = Softmax(W_o * [do_t; c_t(eo, do_t])
$$

Instead, the \textbf{pre-rnn} attention scores are computed based on the \textit{previous} decoder state $do_{t-1}$, instead of the current. 
The resulting context vector is then concatenated with the embedded input $de_t$ of the current decoder step (which is usually the output of the previous decoder step), to produce the decoder input $di_t$.
Note that this makes the input size of the decoder twice as large. 
$$
di_t = [de_t; c_t(eo, do_{t-1})]
$$

The pre-rnn mechanism allows the decoder to incorporate the context information in its recurrency, rather than only using it when generating the output after it. 

\textbf{Full-focus} is a similar mechanism to pre-rnn, but is designed to put more focus on the context vector in comparison to the input word embeddings. This is accomplished by feeding the concatenation through a single feed-forward layer to reduce the dimensionality and an element-wise multiplication with the context-vector.
This reduces the input for the decoder RNN to the original size and is calculated as
$$
di_t = c_t(eo, do_{t-1}) \odot ReLU(W_f * [de_t; c_t(eo, do_{t-1})])
$$

%
%\subsection{Full Focus}
%
%\comment{Introduce/describe/motivate here full focus.}
%Along with the extra loss term, we introduce also a new \textit{gating} attention mechanism, which we call \textit{full-focus}.
%The full-focus attention mechanism is designed to force the decoder to take into account the context vector, by \textit{multiplying} it with the embedded inputs to the decoder, rather than concatenating these two vectors.\\
