# Supplementary material for: Learning compositionally through attentive guidance
Source: arXiv:1805.09657 source file (2019-07-05)
Supplement: Supplementary file 2 [file lookup_table_data.tex]

\section{Lookup table data}

\begin{table}
    \begin{tabular}{l|lc}
        & Example & Size\\
        \hline
    train & t1 t2 011 & 232 \\
    heldout inputs & t1 t2 001 & 40 \\
    heldout compositions & t1 t3 110 & 64 \\
    heldout tables & t1 t8 111 & 192 \\
    new compositions & t7 t8 101 & 32 \\
    \end{tabular}
\end{table}
